# Supplementary material for: Single-view Neural Radiance Fields with Depth Teacher
Source: arXiv:2303.09952 source file (2023-05-11)
Supplement: Supplementary file 1 [file llff_compare2.tex]

\begin{figure*}[th!] \centering
\setlength{\tabcolsep}{0pt}

\begin{tabular}{lcccc}
     \raisebox{2\totalheight}{Plane} &  {\includegraphics[width=0.2\textwidth]{figure/llff compare2/c/DJI_20200226_143918_576_0.JPG}} &  
     {\includegraphics[width=0.2\textwidth]{figure/llff compare2/c/DJI_20200226_143918_576_disp0.JPG}} &  
     {\includegraphics[width=0.2\textwidth]{figure/llff compare2/c/IMG_4044_0.JPG}} & 
     {\includegraphics[width=0.2\textwidth]{figure/llff compare2/c/IMG_4044_disp0.JPG}} \tabularnewline
     
     \raisebox{2\totalheight}{Plane+inpaint} &  
     {\includegraphics[width=0.2\textwidth]{figure/llff compare2/c_inpaint/DJI_20200226_143918_576_0.JPG}} &  
     {\includegraphics[width=0.2\textwidth]{figure/llff compare2/c_inpaint/DJI_20200226_143918_576_disp0.JPG}} &  
     {\includegraphics[width=0.2\textwidth]{figure/llff compare2/c_inpaint/IMG_4044_0.JPG}} & 
     {\includegraphics[width=0.2\textwidth]{figure/llff compare2/c_inpaint/IMG_4044_disp0.JPG}} \tabularnewline
     
     \raisebox{2\totalheight}{Plane+Volume($N = 16$)} &  
     {\includegraphics[width=0.2\textwidth]{figure/llff compare2/f/DJI_20200226_143918_576_0.JPG}} &  
     {\includegraphics[width=0.2\textwidth]{figure/llff compare2/f/DJI_20200226_143918_576_disp0.JPG}} &  
     {\includegraphics[width=0.2\textwidth]{figure/llff compare2/f/IMG_4044_0.JPG}} & 
     {\includegraphics[width=0.2\textwidth]{figure/llff compare2/f/IMG_4044_disp0.JPG}}\tabularnewline
     
     \raisebox{2\totalheight}{Plane+Volume($N = 16$)+inpaint} &  
     {\includegraphics[width=0.2\textwidth]{figure/llff compare2/f_inpaint/DJI_20200226_143918_576_0.JPG}} &  
     {\includegraphics[width=0.2\textwidth]{figure/llff compare2/f_inpaint/DJI_20200226_143918_576_disp0.JPG}} &  
     {\includegraphics[width=0.2\textwidth]{figure/llff compare2/f_inpaint/IMG_4044_0.JPG}}& 
     {\includegraphics[width=0.2\textwidth]{figure/llff compare2/f_inpaint/IMG_4044_disp0.JPG}}\tabularnewline
     
     \raisebox{2\totalheight}{Volume($N = 16$)} &  
     {\includegraphics[width=0.2\textwidth]{figure/llff compare2/fonly/DJI_20200226_143918_576_0.JPG}} &  
     {\includegraphics[width=0.2\textwidth]{figure/llff compare2/fonly/DJI_20200226_143918_576_disp0.JPG}} &  
     {\includegraphics[width=0.2\textwidth]{figure/llff compare2/fonly/IMG_4044_0.JPG}}&
     {\includegraphics[width=0.2\textwidth]{figure/llff compare2/fonly/IMG_4044_disp0.JPG}}\tabularnewline
     
     \raisebox{2\totalheight}{Volume($N = 16$)+inpaint} &  
     {\includegraphics[width=0.2\textwidth]{figure/llff compare2/fonly_inpaint/DJI_20200226_143918_576_0.JPG}} &  
     {\includegraphics[width=0.2\textwidth]{figure/llff compare2/fonly_inpaint/DJI_20200226_143918_576_disp0.JPG}} &  
     {\includegraphics[width=0.2\textwidth]{figure/llff compare2/fonly_inpaint/IMG_4044_0.JPG}}&
     {\includegraphics[width=0.2\textwidth]{figure/llff compare2/fonly_inpaint/IMG_4044_disp0.JPG}}
\end{tabular}
    % \vspace{1pt}
    \caption{importance sampling} 
    \label{fig_kitti_vis}
    % \vspace{-4pt}
\end{figure*}
