# Supplementary material for: Single-view Neural Radiance Fields with Depth Teacher
Source: arXiv:2303.09952 source file (2023-05-11)
Supplement: Supplementary file 2 [file other_method.tex]

\begin{figure*}[t!] \centering
\setlength{\tabcolsep}{1.5pt}
\begin{tabular}{ccccc}
     Input  & PixelSynth & 3D Photo & Ours & GT \\ 
     \includegraphics[width=0.17\textwidth]{figure/other method not nerf/room_src.png}  & 
     \includegraphics[width=0.17\textwidth]{figure/other method not nerf/room_pixel.png} &
     \includegraphics[width=0.17\textwidth]{figure/other method not nerf/DJI_20200226_143855_969.png} &
     \includegraphics[width=0.17\textwidth]{figure/other method not nerf/0029_tgt_imgs_syn.png}& 
     \includegraphics[width=0.17\textwidth]{figure/other method not nerf/0029_tgt_imgs.png}
     \\
     \includegraphics[width=0.17\textwidth]{figure/other method not nerf/horn_src.png} & 
     \includegraphics[width=0.17\textwidth]{figure/other method not nerf/horn_pixel.png} &
     \includegraphics[width=0.17\textwidth]{figure/other method not nerf/DJI_20200223_163031_602.png} &
     \includegraphics[width=0.17\textwidth]{figure/other method not nerf/0015_tgt_imgs_syn.png} & 
     \includegraphics[width=0.17\textwidth]{figure/other method not nerf/0015_tgt_imgs.png}
     \\
\end{tabular}
    \caption{Comparisons other method (PixelSynth \cite{Rockwell_2021_ICCV} and 3D Photography \cite{Shih3DP20}) that do not use NeRF or volume rendering technologies. Our method produce less image distortions (as highlighted by the red windows).} 
    % \vspace{-8pt}
    \label{fig other method}
\end{figure*}
