# Supplementary material for: Single-view Neural Radiance Fields with Depth Teacher
Source: arXiv:2303.09952 source file (2023-05-11)
Supplement: Supplementary file 3 [file realestate_depth.tex]

\begin{figure*}[th!] \centering
 \setlength{\tabcolsep}{1.5pt}
\begin{tabular}{lcccc}
     \raisebox{4\totalheight}{RGB} &  {\includegraphics[width=0.2\textwidth]{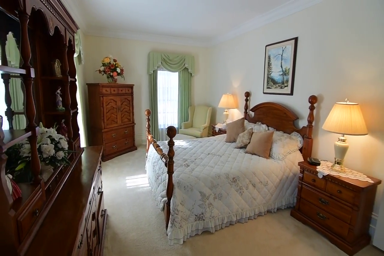}} &  
     {\includegraphics[width=0.2\textwidth]{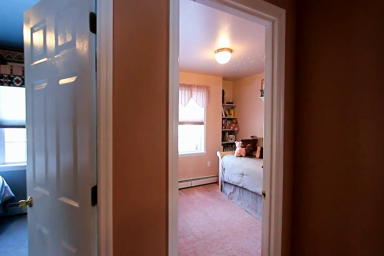}} &  
     {\includegraphics[width=0.2\textwidth]{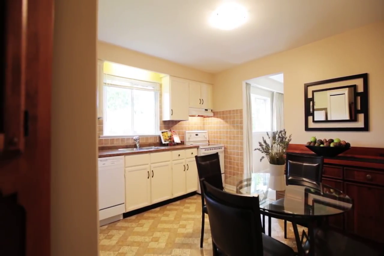}} & 
     {\includegraphics[width=0.2\textwidth]{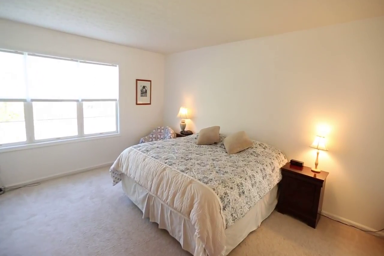}} \tabularnewline
     
     \raisebox{4\totalheight}{MINE} &  
     {\includegraphics[width=0.2\textwidth]{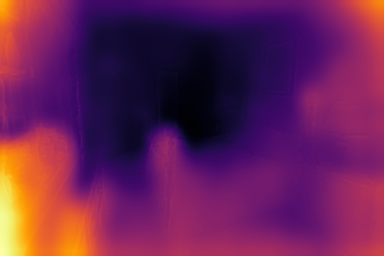}} &  
     {\includegraphics[width=0.2\textwidth]{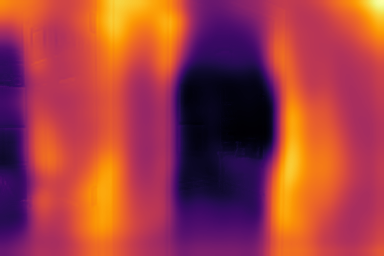}} &  
     {\includegraphics[width=0.2\textwidth]{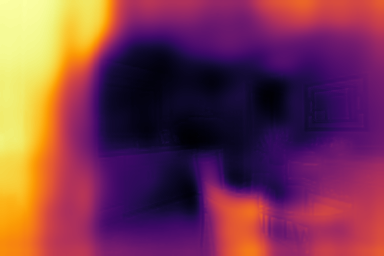}} & 
     {\includegraphics[width=0.2\textwidth]{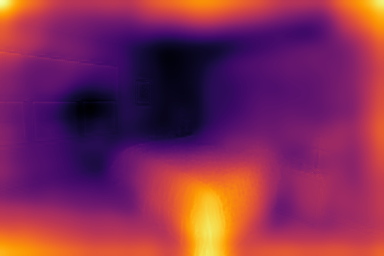}} \tabularnewline
     
     \raisebox{4\totalheight}{Ours} &  
     {\includegraphics[width=0.2\textwidth]{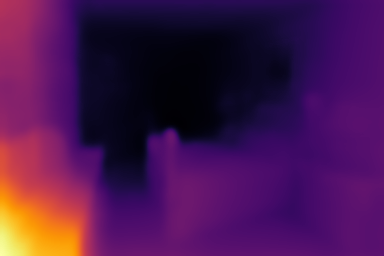}} &  
     {\includegraphics[width=0.2\textwidth]{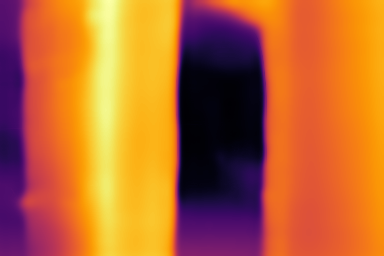}} &  
     {\includegraphics[width=0.2\textwidth]{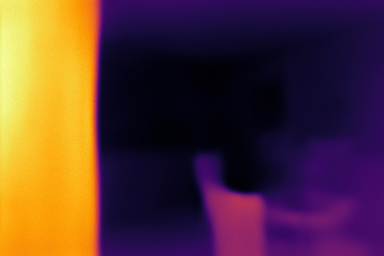}} & 
     {\includegraphics[width=0.2\textwidth]{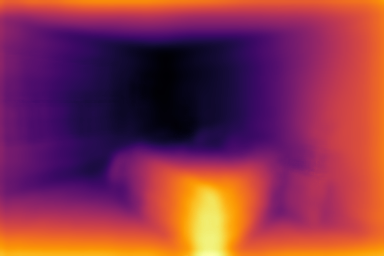}} \tabularnewline
     
\end{tabular}
    % \vspace{1pt}
    \caption{Qualities of depth maps on RealEstate10K dataset. Models are also trained on the RealEstate10K dataset. Our method produces better depth maps with more structure details and sharper depth edges..} 
    \label{fig realestate depth}
    % \vspace{-4pt}
\end{figure*}
