# Supplementary material for: Single-view Neural Radiance Fields with Depth Teacher
Source: arXiv:2303.09952 source file (2023-05-11)
Supplement: Supplementary file 4 [file realestate_inpainting_compare.tex]

\begin{figure*}[t!] \small \centering
\begin{tabular}{ccccc}
     Input & Target GT & MINE\cite{Li_2021_ICCV2} & Ours \\ 
     \includegraphics[width=0.20\textwidth]{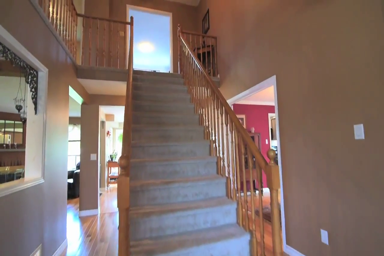} &
     \includegraphics[width=0.20\textwidth]{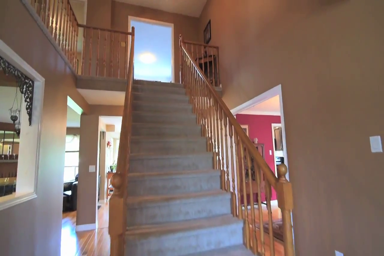} &
     \includegraphics[width=0.20\textwidth]{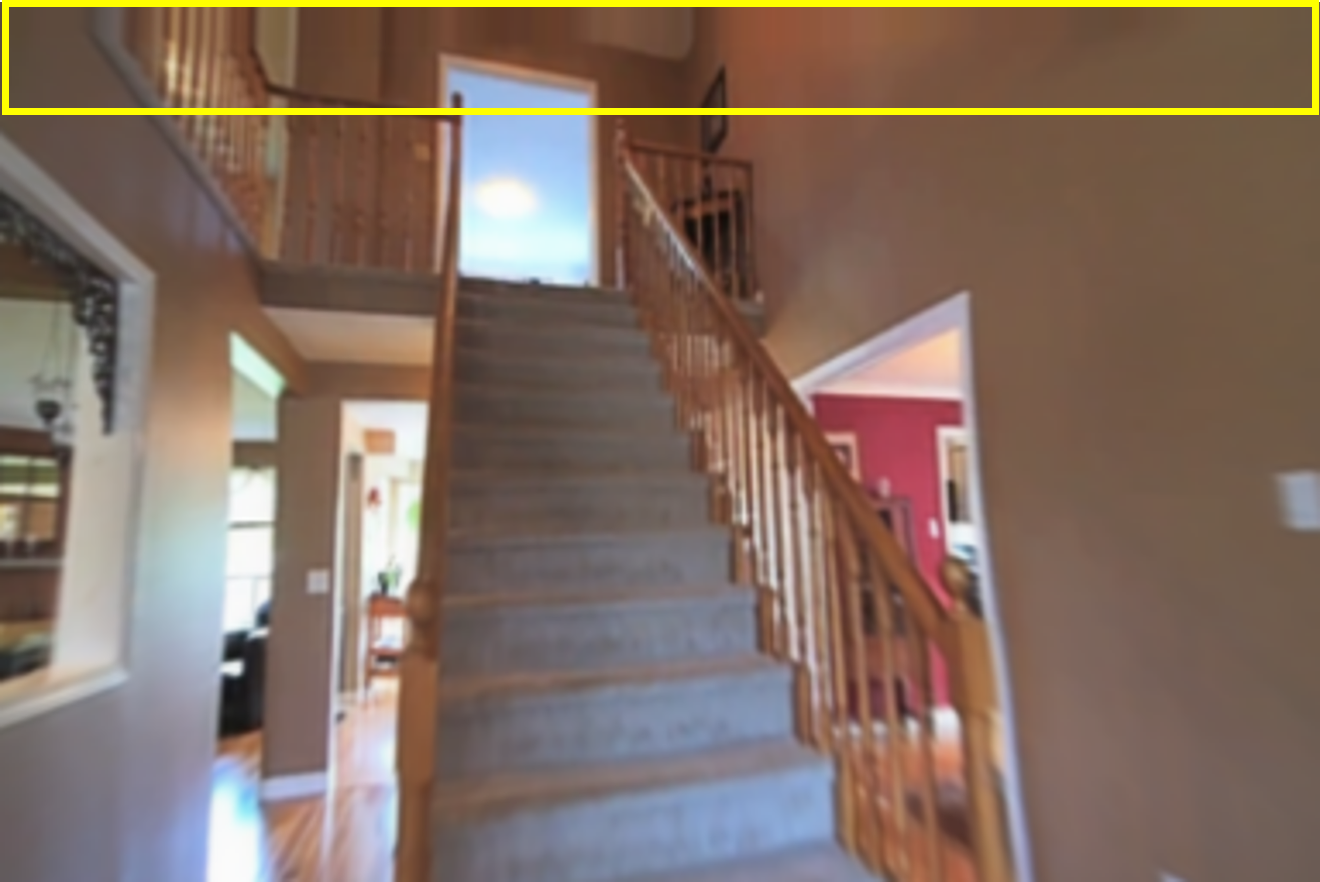} &
     \includegraphics[width=0.20\textwidth]{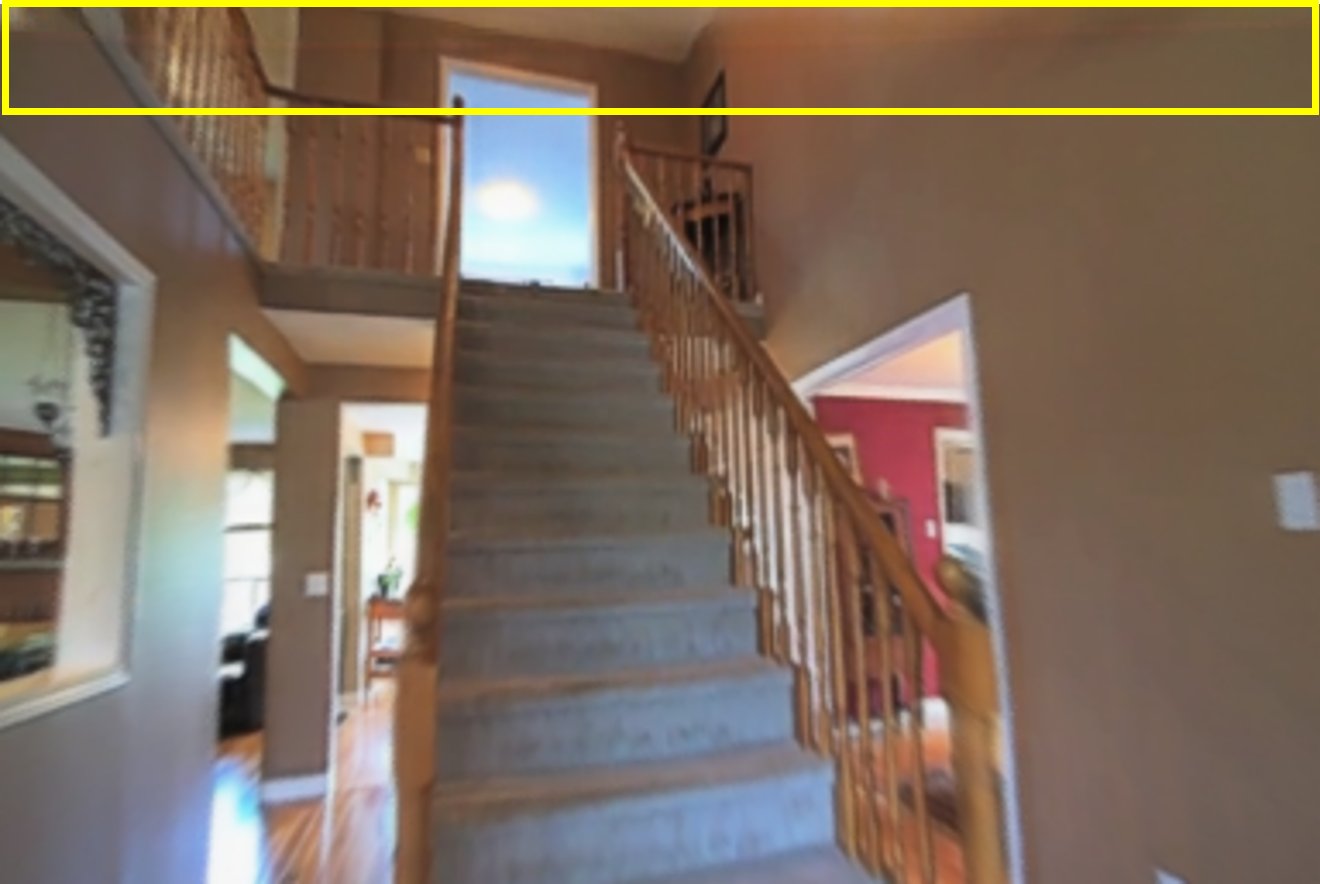} 
     \\
     \includegraphics[width=0.20\textwidth]{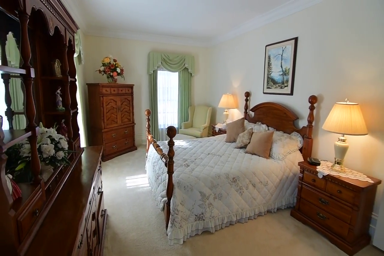} &
     \includegraphics[width=0.20\textwidth]{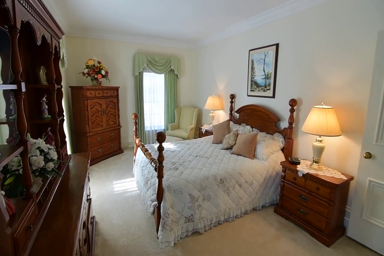} &
     \includegraphics[width=0.20\textwidth]{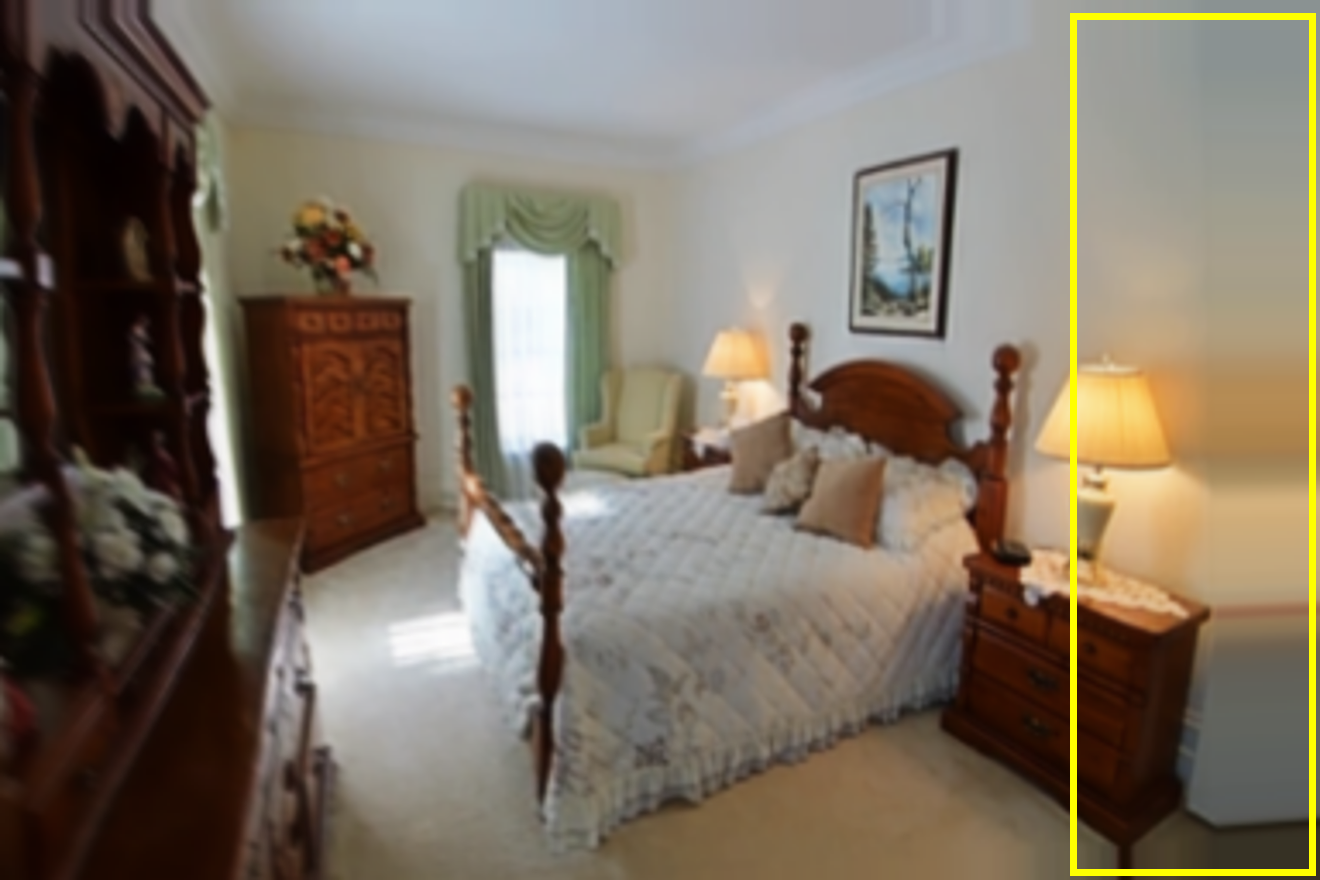} &
     \includegraphics[width=0.20\textwidth]{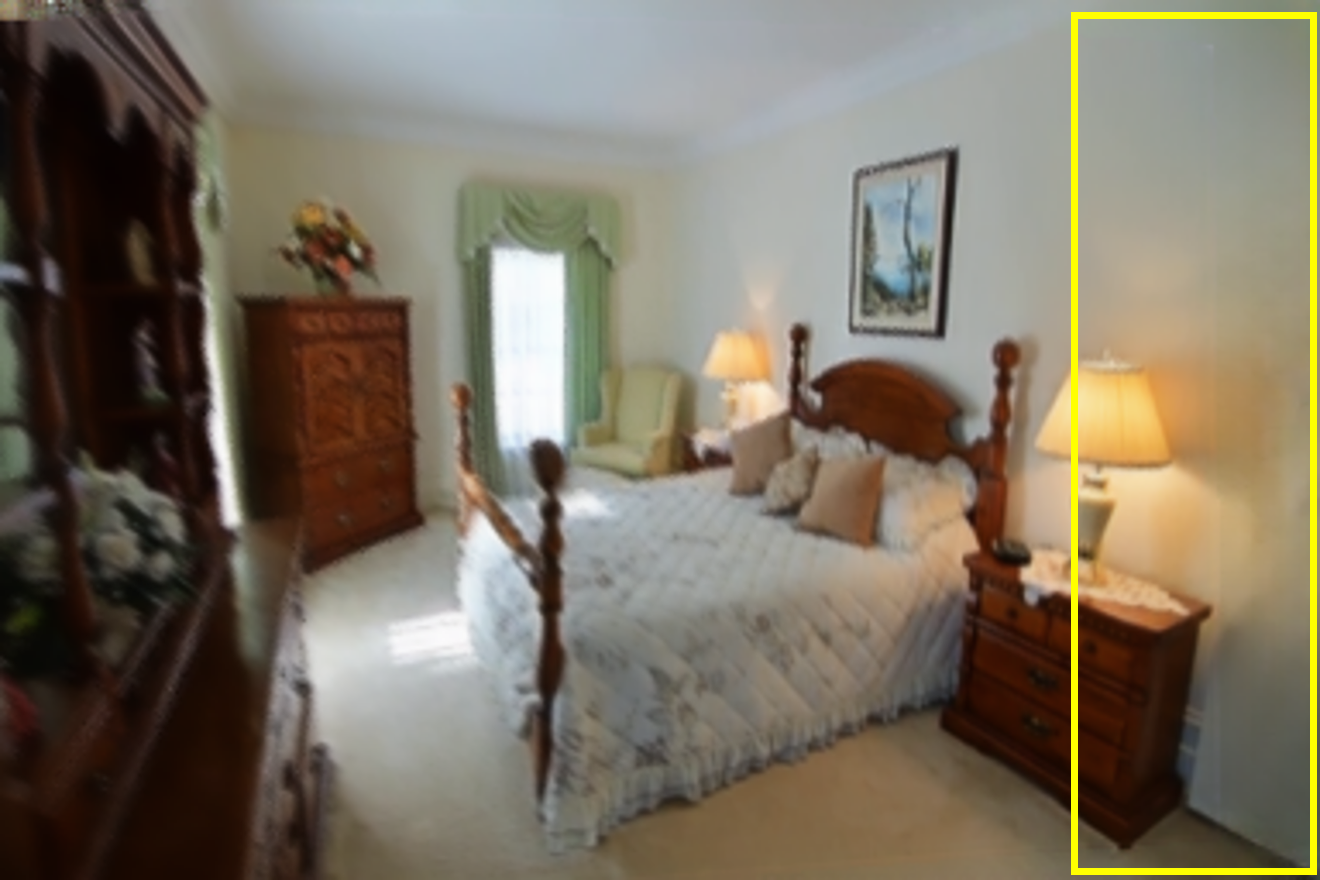} 

\end{tabular}
    \caption{Qualitative comparison on RealEstate10K with \cite{Li_2021_ICCV2}.} 
    \label{fig_realestate_inpaiting}
% \vspace{-4pt}
\end{figure*}
