# Supplementary material for: Single-view Neural Radiance Fields with Depth Teacher
Source: arXiv:2303.09952 source file (2023-05-11)
Supplement: Supplementary file 5 [file sinnerf_2.tex]

\begin{figure*}[h]
\centering
\setlength{\abovecaptionskip}{2pt}
\setlength{\belowcaptionskip}{-8pt}

\subfigure[Input]{
\begin{minipage}[b]{0.20\linewidth}
    \includegraphics[width=1\linewidth]{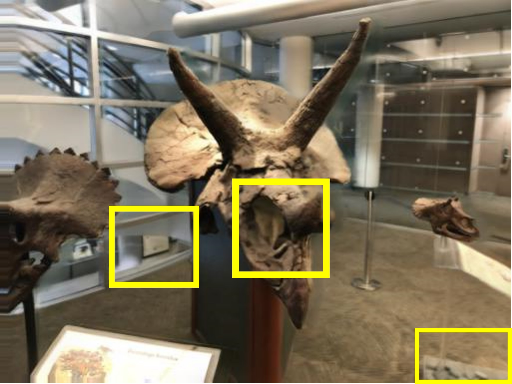}
\end{minipage}
}\hspace{-2mm}
\subfigure[Planar rendering]{
\begin{minipage}[b]{0.20\linewidth}
     \includegraphics[width=1\linewidth]{figure/llff is compare/rgb_nois.png}\\
     \includegraphics[width=1\linewidth]{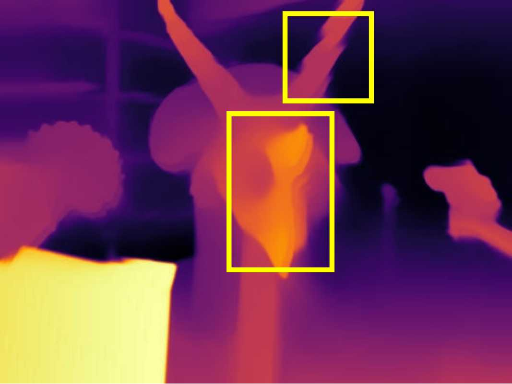} 
\end{minipage}
}\hspace{-2mm}
\subfigure[Planar + volume rendering]{
\begin{minipage}[b]{0.20\linewidth}
     \includegraphics[width=1\linewidth]{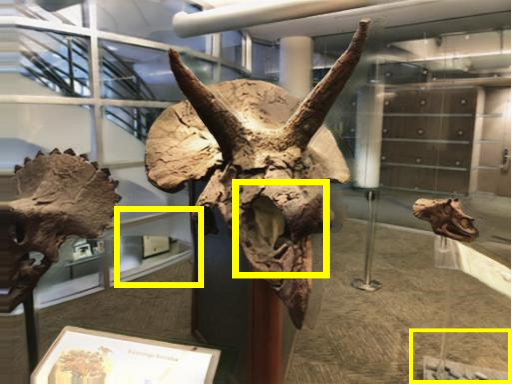}\\
     \includegraphics[width=1\linewidth]{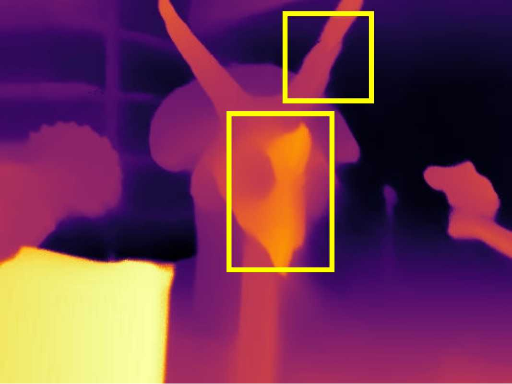}
\end{minipage}
}
%}
    % \vspace{1pt}
    \caption{sinnerf.} 
    \label{fig: llff_room_sinnerf}
    % \vspace{-4pt}
\end{figure*}
