# Supplementary material for: Single-view Neural Radiance Fields with Depth Teacher
Source: arXiv:2303.09952 source file (2023-05-11)
Supplement: Supplementary file 6 [file sinnerf_compare.tex]

\begin{figure*}[t]
\centering

\subfigure[SinNeRF~(PSNR:15.6)]{
\begin{minipage}[b]{0.25\linewidth}
     \includegraphics[width=1\linewidth]{figure/sinnerf compare/DJI_20200226_143852_910_sin.JPG}\\
     \includegraphics[width=1\linewidth]{figure/sinnerf compare/DJI_20200226_143852_910_sin_disp.JPG} 
\end{minipage}
}\hspace{-2mm}
\subfigure[Our method (PSNR:20.1)]{
\begin{minipage}[b]{0.25\linewidth}
     \includegraphics[width=1\linewidth]{figure/sinnerf compare/DJI_20200226_143852_910_ours.JPG}\\
     \includegraphics[width=1\linewidth]{figure/sinnerf compare/DJI_20200226_143852_910_ours_disp.JPG}
\end{minipage}
}
\hspace{-2.7mm}
\subfigure[RGB Ground Truth]{
\begin{minipage}[b]{0.25\linewidth}
     \includegraphics[width=1\linewidth]{figure/sinnerf compare/DJI_20200226_143852_910.JPG}\\[30mm]

\end{minipage}
}
%}
    % \vspace{1pt}
    \caption{Comparision with SinNeRF~\cite{sinnerf}. Models are trained on the NeRF-LLFF dataset and test on the NeRF-LLFF dataset.} 
    \label{fig: sinnerf}
    % \vspace{-4pt}
\end{figure*}
